# Supplementary material for: Covering the Relational Join
Source: arXiv:2003.09537 source file (2020-03-21)
Supplement: Supplementary file 1 [file appendix_dump.tex]

We now consider the following LP (for $1 \le k \le n$):
\begin{align*}
& \min{\sum_{e\in E}x_e}\\
& \text{s.t } \sum_{e \ni v}x_e \ge z_{v}, \text{ for all } v \in V \\
& \sum_{v \in V}z_{v} \ge k \\ 
& z_{v} \le 1, v \in V. \\
& x_e  \ge 0,  e \in E. \numberthis \label{eq:primal}
\end{align*}
We denote the objective value of this LP by $LP_{primal}(G, k)$. We are now ready to prove the following lemma:
\begin{lemma} \label{lemma:galemma1}
For a given query graph $G = (V, E)$ and $k: 1 \le k \le n$, 
\[LP_{primal}(G, k) = LP_{lb}(G, k).\]
\end{lemma}
The proof is in Appendix~\ref{galemma1proof}. Hereon, we would work with LP~\eqref{eq:primal} to reason about $LP_{lb}(G, k)$.
We claim that by making the $z_{v}$s integral, we have a LP that computes $AGM(G, S)$ (which is the AGM bound~\cite{AGM} defined for the subgraph of $G$ defined by $S$). 
Consider the following LP (for $1 \le k \le n$):
\begin{align*}
& \min{\sum_{e\in E}x_e}\\
& \text{s.t } \sum_{e \ni v}x_e \ge z_{v}, \text{ for all } v \in V \\
& \sum_{v \in V}z_{v} \ge k \\ 
& z_{v} = \{0, 1\}, v \in V \\
& x_e  \ge 0,  e \in E.  \numberthis \label{eq:ub}
\end{align*}
We let $LP_{ub}(G, k)$ denote the objective value of the above program. Next, we define what it means to \textit{cover} a vertex.
\begin{definition} [Cover]
A vertex $v \in V$ in LPs \eqref{eq:primal} and \eqref{eq:ub} is considered \textit{cover}ed if and only if $z_{v} = 1$.
\end{definition}

Given Claim~\ref{claim:gaclaim1} and Lemma~\ref{lemma:galemma2}, we are interested in bounding the gap between LP~\eqref{eq:ub} and LP~\eqref{eq:lb} i.e. the value of $LP_{ub}(G, k) - LP_{lb}(G, k)$.
