# Supplementary material for: Covering the Relational Join
Source: arXiv:2003.09537 source file (2020-03-21)
Supplement: Supplementary file 2 [file appendix_sec2.tex]

\section{Missing Details in Section~\ref{section3}}

\subsection{Proof Overview of Theorem~\ref{lowerboundtheorem}}}
We now discuss our case-based analysis briefly. We start by decomposing any $G$ into three subgraphs 
$G_c$, $G_s$ and $G_t$ such that $|V(G)| = |V(G_s)| + |V(G_t)| + |V(G_c)| = n$. Here, $G_s$ is collection of stars of size greater than $1$ and $G_t$ is a collection of singletons. By our decomposition, $G_c = G \setminus \{ G_s \cup G_t\}$. We define $n_s = |V(G_s)|$, $n_t = |V(G_t)|$ and $n_I = \alpha(G_c)$, where $\alpha(G_c)$ denotes the size of the independent set of $G_c$. Let $M$ be a maximum matching on $G$ and $|M|$ denote the total number of vertices in $M$ ($|M|$ is even). We summarize our cases in the form of a table below.
